# Supplementary material for: LakeFM: Toward a Foundation Model for Aquatic Ecosystems Using Irregular Multivariate Multi-depth Time Series Data
Source: arXiv:2606.11268 source file (2026-06-09)
Supplement: Supplementary file 1 [file dataste_procesisng.tex]

\subsection{Dataset Processing for Baselines}

 As the baseline models cannot operate on irregular and sparse data, and the LakeBeD-US data being significantly sparse, we carry out a series of data processing steps. First, we regularize the temporal dimension because the baseline models require regularly sampled inputs. Next, we transform the data into a wide format. Specifically, each variable-depth combination becomes its own column. As a result, each row corresponds to a single timestamp, and all depth-specific measurements are represented as separate features. Next, missing values are handled independently for each column using linear interpolation along the temporal axis. Because the data are converted to variable–depth columns, some columns may have no observations for a particular variable at a given depth. Any column that is completely NaN across all splits (train, validation, and test) is removed. We utilize the these processed data for all the baselines, except, Chronos 2, as it can inherently handle missing values. The reason for performing linear interpolation and not using any deep learning based imputation technique, like SAITS \cite{du2023saits} or CSDI \cite{tashiro2021csdi}, is because, (a) linear interpolation is very common within ecological community, and (b) deep learning imputation models require a lot of training data to be trained before using them for imputing the data. Given the significant amount of sparsity (mostly around 60-70\% and sometimes more), the trained imputation models (tested SAITS) were empirically found to be relatively unstable.
