# Supplementary material for: LakeFM: Toward a Foundation Model for Aquatic Ecosystems Using Irregular Multivariate Multi-depth Time Series Data
Source: arXiv:2606.11268 source file (2026-06-09)
Supplement: Supplementary file 3 [file dataset_details_cam.tex]

\section{Implementation Details}\label{sec:dataset}

\noindent\textbf{In-Distribution (ID) and Out-of-Distribution (OOD) set partitioning.} The lakes are partitioned using a feature-based notion of lake similarity. Each lake is represented by a vector of geographic/physical attributes (latitude, longitude, surface area, mean depth, maximum depth, and elevation). We apply Principal Component Analysis (PCA) to obtain a compact representation capturing the dominant modes of variability across lakes, and perform $k$-means clustering in this normalized feature space, with the number of clusters selected using the silhouette score, favoring clustering that are both tight and well-separated. 
For OOD subset, we select a small set of lakes that are maximally dissimilar from the bulk of the dataset in the learned PCA space. The remaining lakes, which lie in denser regions of the feature space, are treated as ID. For additional information regarding the PCA plots and distribution of lake groups, their ecological state and variables, please refer to the extended version of the paper available here \cite{neog2026lakefm}.
