# Supplementary material for: LakeFM: Toward a Foundation Model for Aquatic Ecosystems Using Irregular Multivariate Multi-depth Time Series Data
Source: arXiv:2606.11268 source file (2026-06-09)
Supplement: Supplementary file 5 [file table_lake_variables_overview.tex]

\begin{table}[t]
\centering
\caption{Overview of available \textbf{2D lake variables} for each lake across all datasets that form the modeling vocabulary of \textsc{LakeFM}.}
\small
\setlength{\tabcolsep}{6pt}

\begin{tabular}{lll}
\toprule
\textbf{Dataset} & \textbf{Lake ID} & \textbf{Available Variables (2D)} \\
\midrule
LakeBedUS & AL   & Water\_DO, WaterTemp, Chla, par \\
LakeBedUS & BVR  & Water\_DO, Water\_DOC, SRP, Water\_TP, WaterTemp \\
LakeBedUS & CRAM & Water\_DO, WaterTemp \\
LakeBedUS & FI   & Water\_DO, WaterTemp \\
LakeBedUS & MO   & Water\_DO, WaterTemp \\
LakeBedUS & BARC & Water\_DO, WaterTemp \\
LakeBedUS & BM   & Water\_DO, WaterTemp, Chla, par \\
LakeBedUS & CB   & Water\_DO, WaterTemp, Chla, par \\
LakeBedUS & CR   & Water\_DO, WaterTemp, Chla, par \\
LakeBedUS & FCR  & Water\_DO, Water\_DOC, SRP, Water\_TP, WaterTemp \\
LakeBedUS & GL4  & Water\_DO, WaterTemp, no3no2, par \\
LakeBedUS & LIRO & Water\_DO, WaterTemp \\
LakeBedUS & ME   & Water\_DO, WaterTemp \\
LakeBedUS & PRLA & Water\_DO, WaterTemp \\
LakeBedUS & PRPO & Water\_DO, WaterTemp \\
LakeBedUS & SP   & Water\_DO, WaterTemp, Chla, par \\
LakeBedUS & SUGG & Water\_DO, WaterTemp \\
LakeBedUS & TB   & Water\_DO, WaterTemp, Chla, par \\
LakeBedUS & TOOK & Water\_DO, WaterTemp \\
LakeBedUS & TR   & Water\_DO, WaterTemp, par \\
LakeBedUS & WI   & Water\_DO, WaterTemp \\
\midrule
WQHansonSim & All &
Water\_DO, Water\_DOC, Water\_POC, Water\_TP \\
\midrule
FcrSimPhy & All &
Chla, WaterTemp, DIN\_ugL \\
\bottomrule
\end{tabular}
\label{tab:variables_per_lake_2d}
\end{table}
