# Supplementary material for: LakeFM: Toward a Foundation Model for Aquatic Ecosystems Using Irregular Multivariate Multi-depth Time Series Data
Source: arXiv:2606.11268 source file (2026-06-09)
Supplement: Supplementary file 6 [file archived_embd_viz.tex]

% \begin{figure*}[t]
%     \centering
%     % ---------- Row 1 ----------
%     \begin{subfigure}[t]{0.32\textwidth}
%         \centering
%         \includegraphics[width=\linewidth]{figures/v_d_masking/CRAM_Masking/NO_MASK_upd_CRAM_plot14.0_evaluation.pdf}
%         \caption{No Masking. CRAM @ 14.0m}
%     \end{subfigure}
%     \hfill
%     \begin{subfigure}[t]{0.32\textwidth}
%         \centering
%         \includegraphics[width=\linewidth]{figures/v_d_masking/CRAM_Masking/MASK_depth_upd_MD_SHL_CRAM_plot14.0_evaluation.pdf}
%         \caption{Shallow Layers Masked. CRAM @ 14.0m}
%     \end{subfigure}
%     \hfill
%     \begin{subfigure}[t]{0.32\textwidth}
%         \centering
%         \includegraphics[width=\linewidth]{figures/v_d_masking/CRAM_Masking/MASK_depth_MD_DEEP_CRAM_plot14.0_evaluation.pdf}
%         \caption{Deeper Layers Masked. CRAM @ 14.0m}
%     \end{subfigure}

%     % ---------- Row 2 ----------
%     \begin{subfigure}[t]{0.32\textwidth}
%         \centering
%         \includegraphics[width=\linewidth]{figures/v_d_masking/CRAM_Masking/NO_MASK_upd_CRAM_plot14.5_evaluation.pdf}
%         \caption{No Masking. CRAM @ 14.5m}
%     \end{subfigure}
%     \hfill
%     \begin{subfigure}[t]{0.32\textwidth}
%         \centering
%         \includegraphics[width=\linewidth]{figures/v_d_masking/CRAM_Masking/MASK_depth_upd_MD_SHL_CRAM_plot14.5_evaluation.pdf}
%         \caption{Shallow Layers Masked. CRAM @ 14.5m}
%     \end{subfigure}
%     \hfill
%     \begin{subfigure}[t]{0.32\textwidth}
%         \centering
%         \includegraphics[width=\linewidth]{figures/v_d_masking/CRAM_Masking/MASK_depth_MD_DEEP_CRAM_plot14.5_evaluation.pdf}
%         \caption{Deeper Layers Masked. CRAM @ 14.5m}
%     \end{subfigure}

%     % ---------- Row 3 ----------
%     \begin{subfigure}[t]{0.32\textwidth}
%         \centering
%         \includegraphics[width=\linewidth]{figures/v_d_masking/CRAM_Masking/NO_MASK_upd_CRAM_plot15.0_evaluation.pdf}
%         \caption{No Masking. CRAM @ 15.0m}
%     \end{subfigure}
%     \hfill
%     \begin{subfigure}[t]{0.32\textwidth}
%         \centering
%         \includegraphics[width=\linewidth]{figures/v_d_masking/CRAM_Masking/MASK_depth_upd_MD_SHL_CRAM_plot15.0_evaluation.pdf}
%         \caption{Shallow Layers Masked. CRAM @ 15.0m}
%     \end{subfigure}
%     \hfill
%     \begin{subfigure}[t]{0.32\textwidth}
%         \centering
%         \includegraphics[width=\linewidth]{figures/v_d_masking/CRAM_Masking/MASK_depth_MD_DEEP_CRAM_plot15.0_evaluation.pdf}
%         \caption{Deeper Layers Masked. CRAM @ 15.0m}
%     \end{subfigure}
%     \caption{Prediction performance visualization in the deeper region under no masking, masking the shallow layers and masking the deeper layers in the input, for Lake CRAM}
%     \label{fig:cram_masking_deep_viz}
% \end{figure*}


% \begin{figure}[htbp]
%     \centering
%     \includegraphics[width=0.48\textwidth]{figures/bl_r2_comparison_lakefm_vs_itransformer.pdf}
%     \caption{Pearson $R^2$ comparison between LakeFM and iTransformer across 100 simulation samples.}
%     \label{fig:bl_lakefm_itrans}
% \end{figure}
% \hfill
% \begin{figure}[htbp]
%     \centering
%     \includegraphics[width=0.48\textwidth]{figures/inversion_rate_comparison_lakefm_vs_itransformer.pdf}
%     \caption{Inversion rate comparison between LakeFM and iTransformer.}
%     \label{fig:inv_lakefm_itrans}
% \end{figure}


% \subsection{Qualitative analysis - Multi-year Lake Embedding Trajectories}

% Figures \ref{fig:trajectories_2014_2017}, \ref{fig:trajectories_2018_2020}, \ref{fig:trajectories_2020_2022} visualize a single lake's temporal evolution across extended time periods (2014-2017, 2018-2020, or 2020-2022). Each trajectory shows the lake's t-SNE projected embeddings, where the x and y axes represent the two t-SNE dimensions. A \textit{red circle} marks the trajectory start point, and the end point. \textit{Yellow diamonds} indicate year transitions (e.g., December 2014 to January 2015), helping identify inter-annual shifts. Arrows along the trajectory show the temporal direction of progression. The color gradient follows a plasma colormap: purple/blue tones represent winter months (January-March), transitioning through pink and orange for spring and summer, and culminating in yellow for late-year months (October-December).


\clearpage

% ========== 2014-2017 Period ==========
% \begin{figure*}[t]
% \centering
% \textbf{Period: 2014--2017}\\[10pt]

% % Row 1: AL and BM
% \begin{minipage}[b]{0.48\linewidth}
% \centering
% \includegraphics[width=\linewidth]{figures/continuous_multi_year/iid_2014_2017/lake_1_AL_continuous_2014_2017.png}
% \caption*{(a) Lake AL}
% \end{minipage}
% \hfill
% \begin{minipage}[b]{0.48\linewidth}
% \centering
% \includegraphics[width=\linewidth]{figures/continuous_multi_year/iid_2014_2017/lake_2_BM_continuous_2014_2017.png}
% \caption*{(b) Lake BM}
% \end{minipage}\\[10pt]

% % Row 2: CB and CR
% \begin{minipage}[b]{0.48\linewidth}
% \centering
% \includegraphics[width=\linewidth]{figures/continuous_multi_year/iid_2014_2017/lake_4_CB_continuous_2014_2017.png}
% \caption*{(c) Lake CB}
% \end{minipage}
% \hfill
% \begin{minipage}[b]{0.48\linewidth}
% \centering
% \includegraphics[width=\linewidth]{figures/continuous_multi_year/iid_2014_2017/lake_5_CR_continuous_2014_2017.png}
% \caption*{(d) Lake CR}
% \end{minipage}\\[10pt]

% % Row 3: FI and SP
% \begin{minipage}[b]{0.48\linewidth}
% \centering
% \includegraphics[width=\linewidth]{figures/continuous_multi_year/iid_2014_2017/lake_8_FI_continuous_2014_2017.png}
% \caption*{(e) Lake FI}
% \end{minipage}
% \hfill
% \begin{minipage}[b]{0.48\linewidth}
% \centering
% \includegraphics[width=\linewidth]{figures/continuous_multi_year/iid_2014_2017/lake_13_SP_continuous_2014_2017.png}
% \caption*{(f) Lake SP}
% \end{minipage}\\[10pt]

% \clearpage


% % Row 4: TB and ME
% \begin{minipage}[b]{0.48\linewidth}
% \centering
% \includegraphics[width=\linewidth]{figures/continuous_multi_year/iid_2014_2017/lake_14_TB_continuous_2014_2017.png}
% \caption*{(g) Lake TB}
% \end{minipage}
% \hfill
% \begin{minipage}[b]{0.48\linewidth}
% \centering
% \includegraphics[width=\linewidth]{figures/continuous_multi_year/plots/ood_2014_2017/lake_3_ME_continuous_2014_2017.png}
% \caption*{(h) Lake ME}
% \end{minipage}\\[10pt]

% % Row 5: TR
% \begin{minipage}[b]{0.48\linewidth}
% \centering
% \includegraphics[width=\linewidth]{figures/continuous_multi_year/plots/ood_2014_2017/lake_6_TR_continuous_2014_2017.png}
% \caption*{(i) Lake TR}
% \end{minipage}

% \caption{Embedding trajectories for all lakes during 2014--2017 period.}
% \label{fig:trajectories_2014_2017}
% \end{figure*}

% \clearpage

% ========== 2014--2017 Period ==========
% ========== 2014--2017 Period ==========
% \begin{figure*}[t]
% \centering
% \textbf{Period: 2014--2017}\\

% \newcommand{\plotheight}{0.22\textheight}

% % ---------- Row 1 ----------
% \begin{minipage}[t]{0.31\linewidth}
% \centering
% \includegraphics[height=\plotheight]{figures/continuous_multi_year/iid_2014_2017/lake_1_AL_continuous_2014_2017.png}
% \caption*{(a) Lake AL}
% \end{minipage}\hfill
% \begin{minipage}[t]{0.31\linewidth}
% \centering
% \includegraphics[height=\plotheight]{figures/continuous_multi_year/iid_2014_2017/lake_2_BM_continuous_2014_2017.png}
% \caption*{(b) Lake BM}
% \end{minipage}
% % \hfill
% \begin{minipage}[t]{0.31\linewidth}
% \centering
% \includegraphics[height=\plotheight]{figures/continuous_multi_year/iid_2014_2017/lake_4_CB_continuous_2014_2017.png}
% \caption*{(c) Lake CB}
% \end{minipage}

% % \vspace{-6pt}

% % ---------- Row 2 ----------
% \begin{minipage}[t]{0.31\linewidth}
% \centering
% \includegraphics[height=\plotheight]{figures/continuous_multi_year/iid_2014_2017/lake_5_CR_continuous_2014_2017.png}
% \caption*{(d) Lake CR}
% \end{minipage}\hfill
% \begin{minipage}[t]{0.31\linewidth}
% \centering
% \includegraphics[height=\plotheight]{figures/continuous_multi_year/iid_2014_2017/lake_8_FI_continuous_2014_2017.png}
% \caption*{(e) Lake FI}
% \end{minipage}\hfill
% \begin{minipage}[t]{0.31\linewidth}
% \centering
% \includegraphics[height=\plotheight]{figures/continuous_multi_year/iid_2014_2017/lake_13_SP_continuous_2014_2017.png}
% \caption*{(f) Lake SP}
% \end{minipage}

% % \vspace{-6pt}

% % ---------- Row 3 ----------
% \begin{minipage}[t]{0.31\linewidth}
% \centering
% \includegraphics[height=\plotheight]{figures/continuous_multi_year/iid_2014_2017/lake_14_TB_continuous_2014_2017.png}
% \caption*{(g) Lake TB}
% \end{minipage}\hfill
% \begin{minipage}[t]{0.31\linewidth}
% \centering
% \includegraphics[height=\plotheight]{figures/continuous_multi_year/plots/ood_2014_2017/lake_3_ME_continuous_2014_2017.png}
% \caption*{(h) Lake ME}
% \end{minipage}\hfill
% \begin{minipage}[t]{0.31\linewidth}
% \centering
% \includegraphics[height=\plotheight]{figures/continuous_multi_year/plots/ood_2014_2017/lake_6_TR_continuous_2014_2017.png}
% \caption*{(i) Lake TR}
% \end{minipage}

% % \vspace{-4pt}

% \caption{Embedding trajectories for all lakes during the 2014--2017 period.}
% \label{fig:trajectories_2014_2017}
% \end{figure*}




% % ========== 2018-2020 Period ==========
% \begin{figure*}[t]
% \centering
% \textbf{Period: 2018--2020}\\[10pt]

% % Row 1: AL and CB
% \begin{minipage}[b]{0.48\linewidth}
% \centering
% \includegraphics[width=\linewidth]{figures/continuous_multi_year/iid_2018_2020/lake_1_AL_continuous_2018_2020.png}
% \caption*{(a) Lake AL}
% \end{minipage}
% \hfill
% \begin{minipage}[b]{0.48\linewidth}
% \centering
% \includegraphics[width=\linewidth]{figures/continuous_multi_year/iid_2018_2020/lake_4_CB_continuous_2018_2020.png}
% \caption*{(b) Lake CB}
% \end{minipage}\\[10pt]

% % Row 2: CR and FI
% \begin{minipage}[b]{0.48\linewidth}
% \centering
% \includegraphics[width=\linewidth]{figures/continuous_multi_year/iid_2018_2020/lake_5_CR_continuous_2018_2020.png}
% \caption*{(c) Lake CR}
% \end{minipage}
% \hfill
% \begin{minipage}[b]{0.48\linewidth}
% \centering
% \includegraphics[width=\linewidth]{figures/continuous_multi_year/iid_2018_2020/lake_8_FI_continuous_2018_2020.png}
% \caption*{(d) Lake FI}
% \end{minipage}\\[10pt]

% % Row 3: SP and TB
% \begin{minipage}[b]{0.48\linewidth}
% \centering
% \includegraphics[width=\linewidth]{figures/continuous_multi_year/iid_2018_2020/lake_13_SP_continuous_2018_2020.png}
% \caption*{(e) Lake SP}
% \end{minipage}
% \hfill
% \begin{minipage}[b]{0.48\linewidth}
% \centering
% \includegraphics[width=\linewidth]{figures/continuous_multi_year/iid_2018_2020/lake_14_TB_continuous_2018_2020.png}
% \caption*{(f) Lake TB}
% \end{minipage}\\[10pt]

% \clearpage


% % Row 4: WI and GL4
% \begin{minipage}[b]{0.48\linewidth}
% \centering
% \includegraphics[width=\linewidth]{figures/continuous_multi_year/iid_2018_2020/lake_15_WI_continuous_2018_2020.png}
% \caption*{(g) Lake WI}
% \end{minipage}
% \hfill
% \begin{minipage}[b]{0.48\linewidth}
% \centering
% \includegraphics[width=\linewidth]{figures/continuous_multi_year/plots/ood_2018_2020/lake_2_GL4_continuous_2018_2020.png}
% \caption*{(h) Lake GL4}
% \end{minipage}\\[10pt]

% % Row 5: ME and TR
% \begin{minipage}[b]{0.48\linewidth}
% \centering
% \includegraphics[width=\linewidth]{figures/continuous_multi_year/plots/ood_2018_2020/lake_3_ME_continuous_2018_2020.png}
% \caption*{(i) Lake ME}
% \end{minipage}
% \hfill
% \begin{minipage}[b]{0.48\linewidth}
% \centering
% \includegraphics[width=\linewidth]{figures/continuous_multi_year/plots/ood_2018_2020/lake_6_TR_continuous_2018_2020.png}
% \caption*{(j) Lake TR}
% \end{minipage}

% \caption{Embedding trajectories for all lakes during 2018--2020 period.}
% \label{fig:trajectories_2018_2020}
% \end{figure*}

% \clearpage
% ========== 2018--2020 Period ==========
% \begin{figure*}[t]
% \centering
% \textbf{Period: 2018--2020}\\

% \newcommand{\plotheight}{0.22\textheight}

% % ---------- Row 1 ----------
% \begin{minipage}[t]{0.31\linewidth}
% \centering
% \includegraphics[height=\plotheight]{figures/continuous_multi_year/iid_2018_2020/lake_1_AL_continuous_2018_2020.png}
% \caption*{(a) Lake AL}
% \end{minipage}
% % \hfill
% \begin{minipage}[t]{0.31\linewidth}
% \centering
% \includegraphics[height=\plotheight]{figures/continuous_multi_year/iid_2018_2020/lake_4_CB_continuous_2018_2020.png}
% \caption*{(b) Lake CB}
% \end{minipage}
% % \hfill
% \begin{minipage}[t]{0.31\linewidth}
% \centering
% \includegraphics[height=\plotheight]{figures/continuous_multi_year/iid_2018_2020/lake_5_CR_continuous_2018_2020.png}
% \caption*{(c) Lake CR}
% \end{minipage}

% % \vspace{-6pt}

% % ---------- Row 2 ----------
% \begin{minipage}[t]{0.31\linewidth}
% \centering
% \includegraphics[height=\plotheight]{figures/continuous_multi_year/iid_2018_2020/lake_8_FI_continuous_2018_2020.png}
% \caption*{(d) Lake FI}
% \end{minipage}
% \begin{minipage}[t]{0.31\linewidth}
% \centering
% \includegraphics[height=\plotheight]{figures/continuous_multi_year/iid_2018_2020/lake_13_SP_continuous_2018_2020.png}
% \caption*{(e) Lake SP}
% \end{minipage}
% % \hfill
% \begin{minipage}[t]{0.31\linewidth}
% \centering
% \includegraphics[height=\plotheight]{figures/continuous_multi_year/iid_2018_2020/lake_14_TB_continuous_2018_2020.png}
% \caption*{(f) Lake TB}
% \end{minipage}

% % \vspace{-6pt}

% % ---------- Row 3 ----------
% \begin{minipage}[t]{0.32\linewidth}
% \centering
% \includegraphics[height=\plotheight]{figures/continuous_multi_year/iid_2018_2020/lake_15_WI_continuous_2018_2020.png}
% \caption*{(g) Lake WI}
% \end{minipage}
% % \hfill
% \begin{minipage}[t]{0.31\linewidth}
% \centering
% \includegraphics[height=\plotheight]{figures/continuous_multi_year/plots/ood_2018_2020/lake_2_GL4_continuous_2018_2020.png}
% \caption*{(h) Lake GL4}
% \end{minipage}
% % \hfill
% \begin{minipage}[t]{0.31\linewidth}
% \centering
% \includegraphics[height=\plotheight]{figures/continuous_multi_year/plots/ood_2018_2020/lake_3_ME_continuous_2018_2020.png}
% \caption*{(i) Lake ME}
% \end{minipage}

% % \vspace{-6pt}

% % ---------- Row 4 (single centered) ----------
% \begin{minipage}[t]{0.31\linewidth}
% \centering
% \includegraphics[height=\plotheight]{figures/continuous_multi_year/plots/ood_2018_2020/lake_6_TR_continuous_2018_2020.png}
% \caption*{(j) Lake TR}
% \end{minipage}

% % \vspace{-4pt}

% \caption{Embedding trajectories for all lakes during the 2018--2020 period.}
% \label{fig:trajectories_2018_2020}
% \end{figure*}

% ========== 2020-2022 Period ==========
% \begin{figure*}[t]
% \centering
% \textbf{Period: 2020--2022}\\[10pt]

% % Row 1: CRAM and FCR
% \begin{minipage}[b]{0.48\linewidth}
% \centering
% \includegraphics[width=\linewidth]{figures/continuous_multi_year/iid_2020_2022/lake_6_CRAM_continuous_2020_2022.png}
% \caption*{(a) Lake CRAM}
% \end{minipage}
% \hfill
% \begin{minipage}[b]{0.48\linewidth}
% \centering
% \includegraphics[width=\linewidth]{figures/continuous_multi_year/iid_2020_2022/lake_7_FCR_continuous_2020_2022.png}
% \caption*{(b) Lake FCR}
% \end{minipage}\\[10pt]

% % Row 2: MO and PRLA
% \begin{minipage}[b]{0.48\linewidth}
% \centering
% \includegraphics[width=\linewidth]{figures/continuous_multi_year/iid_2020_2022/lake_10_MO_continuous_2020_2022.png}
% \caption*{(c) Lake MO}
% \end{minipage}
% \hfill
% \begin{minipage}[b]{0.48\linewidth}
% \centering
% \includegraphics[width=\linewidth]{figures/continuous_multi_year/iid_2020_2022/lake_11_PRLA_continuous_2020_2022.png}
% \caption*{(d) Lake PRLA}
% \end{minipage}\\[10pt]

% % Row 3: PRPO and SP
% \begin{minipage}[b]{0.48\linewidth}
% \centering
% \includegraphics[width=\linewidth]{figures/continuous_multi_year/iid_2020_2022/lake_12_PRPO_continuous_2020_2022.png}
% \caption*{(e) Lake PRPO}
% \end{minipage}
% \hfill
% \begin{minipage}[b]{0.48\linewidth}
% \centering
% \includegraphics[width=\linewidth]{figures/continuous_multi_year/iid_2020_2022/lake_13_SP_continuous_2020_2022.png}
% \caption*{(f) Lake SP}
% \end{minipage}\\[10pt]

% \clearpage


% % Row 4: TB and BARC
% \begin{minipage}[b]{0.48\linewidth}
% \centering
% \includegraphics[width=\linewidth]{figures/continuous_multi_year/iid_2020_2022/lake_14_TB_continuous_2020_2022.png}
% \caption*{(g) Lake TB}
% \end{minipage}
% \hfill
% \begin{minipage}[b]{0.48\linewidth}
% \centering
% \includegraphics[width=\linewidth]{figures/continuous_multi_year/plots/ood_2020_2022/lake_1_BARC_continuous_2020_2022.png}
% \caption*{(h) Lake BARC}
% \end{minipage}\\[10pt]

% % Row 5: GL4 and ME
% \begin{minipage}[b]{0.48\linewidth}
% \centering
% \includegraphics[width=\linewidth]{figures/continuous_multi_year/plots/ood_2020_2022/lake_2_GL4_continuous_2020_2022.png}
% \caption*{(i) Lake GL4}
% \end{minipage}
% \hfill
% \begin{minipage}[b]{0.48\linewidth}
% \centering
% \includegraphics[width=\linewidth]{figures/continuous_multi_year/plots/ood_2020_2022/lake_3_ME_continuous_2020_2022.png}
% \caption*{(j) Lake ME}
% \end{minipage}\\[10pt]

% % Row 6: SUGG and TOOK
% \begin{minipage}[b]{0.48\linewidth}
% \centering
% \includegraphics[width=\linewidth]{figures/continuous_multi_year/plots/ood_2020_2022/lake_4_SUGG_continuous_2020_2022.png}
% \caption*{(k) Lake SUGG}
% \end{minipage}
% \hfill
% \begin{minipage}[b]{0.48\linewidth}
% \centering
% \includegraphics[width=\linewidth]{figures/continuous_multi_year/plots/ood_2020_2022/lake_5_TOOK_continuous_2020_2022.png}
% \caption*{(l) Lake TOOK}
% \end{minipage}

% \caption{Embedding trajectories for all lakes during 2020--2022 period.}
% \label{fig:trajectories_2020_2022}
% \end{figure*}
% ========== 2020--2022 Period ==========
% \begin{figure*}[t]
% \centering
% \textbf{Period: 2020--2022}\\

% \newcommand{\plotheight}{0.18\textheight}

% % ---------- Row 1 ----------
% \begin{minipage}[t]{0.31\linewidth}
% \centering
% \includegraphics[height=\plotheight]{figures/continuous_multi_year/iid_2020_2022/lake_6_CRAM_continuous_2020_2022.png}
% \caption*{(a) Lake CRAM}
% \end{minipage}
% \begin{minipage}[t]{0.31\linewidth}
% \centering
% \includegraphics[height=\plotheight]{figures/continuous_multi_year/iid_2020_2022/lake_7_FCR_continuous_2020_2022.png}
% \caption*{(b) Lake FCR}
% \end{minipage}
% \begin{minipage}[t]{0.31\linewidth}
% \centering
% \includegraphics[height=\plotheight]{figures/continuous_multi_year/iid_2020_2022/lake_10_MO_continuous_2020_2022.png}
% \caption*{(c) Lake MO}
% \end{minipage}

% % ---------- Row 2 ----------
% \begin{minipage}[t]{0.31\linewidth}
% \centering
% \includegraphics[height=\plotheight]{figures/continuous_multi_year/iid_2020_2022/lake_11_PRLA_continuous_2020_2022.png}
% \caption*{(d) Lake PRLA}
% \end{minipage}
% \begin{minipage}[t]{0.31\linewidth}
% \centering
% \includegraphics[height=\plotheight]{figures/continuous_multi_year/iid_2020_2022/lake_12_PRPO_continuous_2020_2022.png}
% \caption*{(e) Lake PRPO}
% \end{minipage}
% \begin{minipage}[t]{0.31\linewidth}
% \centering
% \includegraphics[height=\plotheight]{figures/continuous_multi_year/iid_2020_2022/lake_13_SP_continuous_2020_2022.png}
% \caption*{(f) Lake SP}
% \end{minipage}

% % ---------- Row 3 ----------
% \begin{minipage}[t]{0.31\linewidth}
% \centering
% \includegraphics[height=\plotheight]{figures/continuous_multi_year/iid_2020_2022/lake_14_TB_continuous_2020_2022.png}
% \caption*{(g) Lake TB}
% \end{minipage}
% % \hfill
% \begin{minipage}[t]{0.31\linewidth}
% \centering
% \includegraphics[height=\plotheight]{figures/continuous_multi_year/plots/ood_2020_2022/lake_1_BARC_continuous_2020_2022.png}
% \caption*{(h) Lake BARC}
% \end{minipage}
% % \hfill
% \begin{minipage}[t]{0.31\linewidth}
% \centering
% \includegraphics[height=\plotheight]{figures/continuous_multi_year/plots/ood_2020_2022/lake_2_GL4_continuous_2020_2022.png}
% \caption*{(i) Lake GL4}
% \end{minipage}

% % \vspace{-6pt}

% % ---------- Row 4 ----------
% \begin{minipage}[t]{0.31\linewidth}
% \centering
% \includegraphics[height=\plotheight]{figures/continuous_multi_year/plots/ood_2020_2022/lake_3_ME_continuous_2020_2022.png}
% \caption*{(j) Lake ME}
% \end{minipage}
% % \hfill
% \begin{minipage}[t]{0.31\linewidth}
% \centering
% \includegraphics[height=\plotheight]{figures/continuous_multi_year/plots/ood_2020_2022/lake_4_SUGG_continuous_2020_2022.png}
% \caption*{(k) Lake SUGG}
% \end{minipage}
% % \hfill
% \begin{minipage}[t]{0.31\linewidth}
% \centering
% \includegraphics[height=\plotheight]{figures/continuous_multi_year/plots/ood_2020_2022/lake_5_TOOK_continuous_2020_2022.png}
% \caption*{(l) Lake TOOK}
% \end{minipage}

% % \vspace{-4pt}

% \caption{Embedding trajectories for all lakes during the 2020--2022 period.}
% \label{fig:trajectories_2020_2022}
% \end{figure*}

% \subsection{Lake Pair Trajectories}
% Figures \ref{fig:lake_pairs_1}, \ref{fig:lake_pairs_2}, \ref{fig:lake_pairs_3} compare lakes in pairs within a single year (2018-2022). The \textit{colored circles} mark where each lake begins, and \textit{colored squares} mark where each lake ends, with colors matching each lake's designated trajectory color. Trajectories are composed of t-SNE projected embeddings plotted along x and y axes. Arrows embedded in each trajectory indicate temporal progression throughout the year. The plasma colormap overlay on each trajectory follows the same seasonal pattern: purple for early-year months transitioning to yellow for late-year months. This visualization enables direct comparison of seasonal dynamics and ecological state similarities between different lakes.


% \clearpage

% % ========== Lake Pair Comparisons ==========
% \begin{figure*}[t]
% \centering
% \newcommand{\plotheight}{0.18\textheight}
% % Row 1: BARC_ME and BARC_SUGG
% \begin{minipage}[t]{0.32\linewidth}
% \centering
% \includegraphics[height=\plotheight]{figures/all_lake_pairs/barc_me_2022.png}
% \caption*{(a) BARC vs ME (2022)}
% \end{minipage}
% % \hfill
% \begin{minipage}[t]{0.32\linewidth}
% \centering
% \includegraphics[height=\plotheight]{figures/all_lake_pairs/barc_sugg_2022.png}
% \caption*{(b) BARC vs SUGG (2022)}
% \end{minipage}
% \begin{minipage}[t]{0.32\linewidth}
% \centering
% \includegraphics[height=\plotheight]{figures/all_lake_pairs/bm_cb_2022.png}
% \caption*{(c) BM vs CB (2022)}
% \end{minipage}
% % Row 2: 

% \begin{minipage}[b]{0.32\linewidth}
% \centering
% \includegraphics[height=\plotheight]{figures/all_lake_pairs/bm_cb_2021.png}
% \caption*{(d) BM vs CB (2021)}
% \end{minipage}
% \begin{minipage}[b]{0.32\linewidth}
% \centering
% \includegraphics[height=\plotheight]{figures/all_lake_pairs/bm_cb_2020.png}
% \caption*{(e) BM vs CB (2020)}
% \end{minipage}
% \begin{minipage}[b]{0.32\linewidth}
% \centering
% \includegraphics[width=\linewidth]{figures/all_lake_pairs/bm_cb_2019.png}
% \caption*{(f) BM vs CB (2019)}
% \end{minipage}

% % Row 4: 
% \begin{minipage}[b]{0.32\linewidth}
% \centering
% \includegraphics[height=\plotheight]{figures/all_lake_pairs/bm_cb_2018.png}
% \caption*{(g) BM vs CB (2018)}
% \end{minipage}
% \begin{minipage}[b]{0.32\linewidth}
% \centering
% \includegraphics[height=\plotheight]{figures/all_lake_pairs/cr_bm_2022.png}
% \caption*{(h) CR vs BM (2022)}
% \end{minipage}

% \caption{Lake pair trajectory comparisons (Part 1).}
% \label{fig:lake_pairs_1}
% \end{figure*}

% \clearpage

% % ========== Continued Figure ==========
% \begin{figure*}[t]
% % \ContinuedFloat
% \newcommand{\plotheight}{0.18\textheight}
% \centering

% % Row 5: CR_BM continued
% \begin{minipage}[t]{0.32\linewidth}
% \centering
% \includegraphics[height=\plotheight]{figures/all_lake_pairs/cr_bm_2021.png}
% \caption*{(i) CR vs BM (2021)}
% \end{minipage}
% \begin{minipage}[t]{0.32\linewidth}
% \centering
% \includegraphics[height=\plotheight]{figures/all_lake_pairs/cr_bm_2019.png}
% \caption*{(j) CR vs BM (2019)}
% \end{minipage}
% \begin{minipage}[t]{0.32\linewidth}
% \centering
% \includegraphics[height=\plotheight]{figures/all_lake_pairs/cr_bm_2018.png}
% \caption*{(k) CR vs BM (2018)}
% \end{minipage}


% \begin{minipage}[t]{0.32\linewidth}
% \centering
% \includegraphics[height=\plotheight]{figures/all_lake_pairs/cr_cb_2022.png}
% \caption*{(l) CR vs CB (2022)}
% \end{minipage}
% \begin{minipage}[t]{0.32\linewidth}
% \centering
% \includegraphics[height=\plotheight]{figures/all_lake_pairs/cr_cb_2021.png}
% \caption*{(m) CR vs CB (2021)}
% \end{minipage}
% \begin{minipage}[t]{0.32\linewidth}
% \centering
% \includegraphics[height=\plotheight]{figures/all_lake_pairs/cr_sp_2022.png}
% \caption*{(n) CR vs SP (2022)}
% \end{minipage}\\[10pt]


% \begin{minipage}[t]{0.32\linewidth}
% \centering
% \includegraphics[height=\plotheight]{figures/all_lake_pairs/cr_sp_2021.png}
% \caption*{(o) CR vs SP (2021)}
% \end{minipage}
% \begin{minipage}[t]{0.32\linewidth}
% \centering
% \includegraphics[height=\plotheight]{figures/all_lake_pairs/cr_sp_2019.png}
% \caption*{(p) CR vs SP (2019)}
% \end{minipage}

% \caption{Lake pair trajectory comparisons (Part 2).}
% \label{fig:lake_pairs_2}
% \end{figure*}

% \clearpage

% % ========== Continued Figure ==========
% \begin{figure*}[t]
% % \ContinuedFloat
% \newcommand{\plotheight}{0.17\textheight}
% \centering

% % Row 9: CR_SP and FI_BM
% \begin{minipage}[t]{0.32\linewidth}
% \centering
% \includegraphics[height=\plotheight]{figures/all_lake_pairs/cr_sp_2018.png}
% \caption*{(q) CR vs SP (2018)}
% \end{minipage}
% \begin{minipage}[t]{0.32\linewidth}
% \centering
% \includegraphics[height=\plotheight]{figures/all_lake_pairs/fi_bm_2022.png}
% \caption*{(r) FI vs BM (2022)}
% \end{minipage}
% \begin{minipage}[t]{0.32\linewidth}
% \centering
% \includegraphics[height=\plotheight]{figures/all_lake_pairs/fi_cb_2022.png}
% \caption*{(s) FI vs CB (2022)}
% \end{minipage}


% \begin{minipage}[t]{0.32\linewidth}
% \centering
% \includegraphics[height=\plotheight]{figures/all_lake_pairs/fi_cr_2022.png}
% \caption*{(t) FI vs CR (2022)}
% \end{minipage}
% \begin{minipage}[t]{0.32\linewidth}
% \centering
% \includegraphics[height=\plotheight]{figures/all_lake_pairs/fi_sp_2022.png}
% \caption*{(u) FI vs SP (2022)}
% \end{minipage}
% \begin{minipage}[t]{0.32\linewidth}
% \centering
% \includegraphics[height=\plotheight]{figures/all_lake_pairs/liro_bm_2022.png}
% \caption*{(v) LIRO vs BM (2022)}
% \end{minipage}\\[10pt]

% % Row 12: LIRO_CB and SP_CB
% \begin{minipage}[t]{0.32\linewidth}
% \centering
% \includegraphics[height=\plotheight]{figures/all_lake_pairs/liro_cb_2022.png}
% \caption*{(w) LIRO vs CB (2022)}
% \end{minipage}
% \begin{minipage}[t]{0.32\linewidth}
% \centering
% \includegraphics[height=\plotheight]{figures/all_lake_pairs/sp_cb_2022.png}
% \caption*{(x) SP vs CB (2022)}
% \end{minipage}
% \begin{minipage}[t]{0.32\linewidth}
% \centering
% \includegraphics[height=\plotheight]{figures/all_lake_pairs/sp_cb_2021.png}
% \caption*{(y) SP vs CB (2021)}
% \end{minipage}


% \begin{minipage}[t]{0.32\linewidth}
% \centering
% \includegraphics[height=\plotheight]{figures/all_lake_pairs/sp_cb_2019.png}
% \caption*{(z) SP vs CB (2019)}
% \end{minipage}
% \begin{minipage}[t]{0.32\linewidth}
% \centering
% \includegraphics[height=\plotheight]{figures/all_lake_pairs/sp_cb_2018.png}
% \caption*{(aa) SP vs CB (2018)}
% \end{minipage}

% \caption{Lake pair trajectory comparisons (Part 3).}
% \label{fig:lake_pairs_3}
% \end{figure*}

% \clearpage



%%%%%%%%%%%%%%%%%%%%%%%%%%%%%%%
% \subsection{Lake Embedding trajectories based on single input variable}

% Figure \ref{fig:variable_masking} demonstrates the impact of variable masking on learned lake embeddings by comparing three scenarios side-by-side within a single figure. Each subplot displays a lake's trajectory for a specific year as t-SNE projected embeddings along x and y axes. The \textbf{left subplot} shows the baseline trajectory using all available variables (temperature, dissolved oxygen, and metadata), the \textbf{middle subplot} shows the trajectory when dissolved oxygen (DO) is masked (temperature-only model), and the \textbf{right subplot} shows the trajectory when temperature is masked (DO-only model). Arrows embedded in each trajectory indicate temporal progression throughout the year. The plasma colormap provides seasonal context: \textbf{purple tones represent winter/early months (January-March)} transitioning to \textbf{yellow tones for fall/late months (October-December)}. A \textbf{colored circle} marks each trajectory's start point, while a \textbf{colored square} marks the end point. By comparing trajectory shapes and positions across the three subplots, we can assess which variables contribute most to seasonal patterns and ecological state representation in the embedding space.

% \clearpage

% % ========== Variable Masking Analysis ==========
% \begin{figure*}[t]
% \centering

% % Row 1: AL_variable_masking
% \begin{minipage}[b]{0.48\linewidth}
% \centering
% \includegraphics[width=\linewidth]{figures/variate_masking/AL_variable_masking_2022_2022.png}
% \caption*{(a) Lake AL - Variable Masking (2022)}
% \end{minipage}
% \hfill
% \begin{minipage}[b]{0.48\linewidth}
% \centering
% \includegraphics[width=\linewidth]{figures/variate_masking/AL_variable_masking_2021_2021.png}
% \caption*{(b) Lake AL - Variable Masking (2021)}
% \end{minipage}\\[10pt]

% % Row 2: MO_variable_masking
% \begin{minipage}[b]{0.48\linewidth}
% \centering
% \includegraphics[width=\linewidth]{figures/variate_masking/MO_variable_masking_2021_2021.png}
% \caption*{(c) Lake MO - Variable Masking (2021)}
% \end{minipage}
% \hfill
% \begin{minipage}[b]{0.48\linewidth}
% \centering
% \includegraphics[width=\linewidth]{figures/variate_masking/MO_variable_masking_2018_2018.png}
% \caption*{(d) Lake MO - Variable Masking (2018)}
% \end{minipage}


% \begin{minipage}[b]{0.48\linewidth}
% \centering
% \includegraphics[width=\linewidth]{figures/variate_masking/CB_variable_masking_2018_2018.png}
% \caption*{(c) Lake CB - Variable Masking (2018)}
% \end{minipage}
% \hfill
% \begin{minipage}[b]{0.48\linewidth}
% \centering
% \includegraphics[width=\linewidth]{figures/variate_masking/CRAM_variable_masking_2021_2021.png}
% \caption*{(d) Lake CRAM - Variable Masking (2021)}
% \end{minipage}



% \caption{Variable masking analysis showing trajectory changes when DO or Temperature variables are masked. Each plot compares baseline (all variables) against scenarios where either DO or Temperature is ignored.}
% \label{fig:variable_masking}
% \end{figure*}
%%%%%%%%%%%%%%%%%%%%%%%%%%%%%%%%%%%%%%%%%
% \subsection{Lake Embedding Visualization}


% Analysis of lake embeddings over a single year (Figure \ref{fig:iid_2021} reveals that regional similarities are preserved throughout the seasonal cycle. Consistent Seasonal Patterns are observed - lakes from the same region (e.g., the Wisconsin group) exhibit synchronized trajectory patterns through the embedding space. Similarly, we see the North Dakota lakes (PRPO and PRLA) demonstrate distinct, parallel behaviors. Altogether, we think that LakeFM holds much promise for providing valuable insights for limnologists in future work.
% \begin{figure}[htbp]
%     \centering
%     \includegraphics[width=0.4\textwidth]{figures/iid_7lakes_2021_refined.png}
%     \caption{IID Lakes 2021}
%     \label{fig:iid_2021}
% \end{figure}


% \begin{figure}[htbp]
%     \centering
%     \begin{subfigure}{0.48\textwidth}
%         \centering
%         \includegraphics[width=\linewidth]{figures/me_multiyear_2020_2022.png}
%         \subcaption{ME Multi-Year Trajectories}
%         \label{fig:me_multiyear}
%     \end{subfigure}
%     \hfill
%     \begin{subfigure}{0.48\textwidth}
%         \centering
%         \includegraphics[width=\linewidth]{figures/sugg_multiyear_2020_2022.png}
%         \subcaption{SUGG Multi-Year Trajectories}
%         \label{fig:sugg_multiyear}
%     \end{subfigure}
%     \caption{Multi-year trajectories across lakes.}
%     \label{fig:multiyear_trajectories}
% \end{figure}


% \newpage

% \newpage
